# Supplementary material for: Scalable Polyhedral Verification of Recurrent Neural Networks
Source: arXiv:2005.13300 source file (2021-06-10)
Supplement: Supplementary file 1 [file appendix.tex]

\appendix

\section{Comparison with POPQORN based on hash tables}
\label{sec:appendix-popqorn-hashset}

One way to make the prior work POPQORN more scalable is using a hash table. The idea is to store the coefficients of the bounding planes approximating the binary functions computed by POPQORN in the table indexed by the intervals $[l_x,u_x]$ and $[l_y,u_y]$ of the input variables $x$ and $y$. For our benchmarks both $x$ and $y$ are usually in the range $[-2,2]$. The keys $l_x, u_x, l_y,u_y$ in the table are such that $l_x$, $u_x$, $l_y$, $u_y$, $u_x-l_x$ and $u_y-l_y$ are all divisible by a constant $\delta \in \mathbb{R}$. The coefficients for any missing entry $[l'_x,u'_x]$, $[l'_y,u'_y]$ in our table is obtained by finding the smallest intervals in the table $[l_x,u_x]$, $[l_y,u_y]$ containing $[l'_x,u'_x]$ and $[l'_y,u'_y]$ respectively. Our construction ensures that such intervals always exist.

While this approach speeds up POPQORN, it comes at a cost of extra memory and further loss of precision in practice.
There are already 672,400 different cases within the domain $[-2, 2] \times [-2, 2]$ with $\delta=0.1$ which significantly increases memory footprint. Decreasing the value of $\delta=0.01$ improves the precision of the combination but also exponentially increases the size of the table making it computationally prohibitive.
The drop in the precision of certification is noticeable: POPQORN proves 79.2\% out of 500 test data perturbed at frame 7 with $\epsilon=0.05$ while combining it with hash table proves 76.0\%.
We note that in comparison the $\epsilon$ values for every frame proven by \tool are almost twice as large as for POPQORN.
